# Supplementary material for: Machine Learning Percolation Model
Source: arXiv:2101.08928 source file (2021-01-22)
Supplement: Supplementary file 1 [file PRR_supplementary.pdf]

# Supplementary Material: Machine Learning Percolation Model

Shu Cheng[1], Huai Zhang,* and Yaolin Shi
*Key Laboratory of Computational Geodynamics, College of Earth and Planetary Sciences, University of Chinese Academy of Sciences, No.19(A) Yuquan Road, Shijingshan District, Beijing 100049, China*

Fei He[1] and Ka-Di Zhu†
*Key Laboratory of Artificial Structures and Quantum Control (Ministry of Education), School of Physics and Astronomy, Shanghai Jiao Tong University, 800 Dong Chuan Road, Shanghai 200240, China*

## I. DESCRIPTION OF THE TECHNICAL TERMS OF MACHINE LEARNING AND THEIR ALGORITHMS

In this section, we will delivers more details about the technical terms of machine learning and their algorithms that we used in Tensorflow 2.2 and scikit-learn 0.23.

### A. The technical terms of machine learning

**Activation function.** To make convolutional neural networks (CNNs) learn complex decision boundary, a non-linear activation function is applied in some layers. The most common activation functions include sigmoid, tanh, ReLU (Rectified Linear Unit), and their variants.

**Loss function.** CNNs takes certain indicator as a clue to find the optimal model while training. The indicator is loss function. Usually, loss function can be expressed by many function, such as mean square error, cross-entropy error, and so on.

**Optimizer.** Optimizer refers to update parameters in right direction in the process of training. Thus, loss function continuously approaches the global minimum. The most common optimizer include stochastic gradient descent (SGD), momentum, Adagrad, and Adam.

**Mini-Batch.** Mini-batching is a technique that applies small parts of training dataset at a time rather than the entire training set. It enables models to be trained on computers with small memory.

**Epoch.** An epoch is the process of training all the training dataset at once.

**Regularization.** To reduce generalization error, regularization methods can be used to modify the way of training models. The most common optimizer include L1 regularization and L2 regularization.

**Learning Rate.** Learning rate can control how much the weights are adjusted to gradient loss. The lower the value is, the slower it will go down slower the gradients.

**Dropout.** Dropout is a regularization technique for CNNs to prevent overfitting. It hinders co-adaptation by randomly setting a small fraction of neurons to zero in each training iteration. Dropout layer is used in CNNs and recurrent CNNs.

**Batch Normalization.** Batch normalization is a technique for standardizing inputs of layer in small batches. It can speed up the training process and be used as a regularizer. Batch normalization has been found to be very efficient in CNNs and feedforward networks, but it has not been successfully applied to recurrent CNNs.

---

* hzhang@ucas.ac.cn
† zhukadi@sjtu.edu.cn

**Max-Pooling.** Max-Pooling are usually used in CNNs. A maximum pooling layer picks the maximum from a block of features. Like convolution layer, pooling layer is parameterized by block size and step size. The pooling layer reduces the dimension of representation by retaining the most prominent information. Pooling layer is usually placed between two adjacent convolution layers.

### B. Machine learning algorithms

Our algorithms contain four CNNs, one variational autoencoder (VAE), one convolutional VAE (cVAE), one principal component analysis (PCA), and one $k$-means. These algorithms can generally be separated into 5 categories: regression models (3 algorithms), binary classification models (1 algorithm), generation models (2 algorithms), dimensional reduction method (1 algorithm), and clustering model (1 algorithm). Table S. I shows a list of the machine learning algorithms. Though the principle of each algorithm goes beyond the scope of this article, we still give a brief introduction for each category and gain insightful advantages of the algorithms within different categories.

TABLE S. I: 5 categories for the machine learning algorithms.

| Categories | Algorithms | Purpose |
|---|---|---|
| Regression models | CNNs-I | Simulate the order parameter $\Pi(\boldsymbol{p}, L)$ |
| | CNNs-II | Simulate the order parameter $P(\boldsymbol{p}, L)$ |
| | CNNs-III | Simulate the permeabilities $\boldsymbol{p}$ |
| Binary Classification Models | CNNs-IV | Deduce a new parameter and the critical transition point |
| Generation models | variational autoencoder (VAE) | Generate new configuration $\hat{\boldsymbol{X}}_{\mathrm{VAE}}$ |
| | convolutional VAE (cVAE) | Generate new configuration $\hat{\boldsymbol{X}}_{\mathrm{cVAE}}$ |
| Dimensional reduction method | PCA | Deduce the first principal component |
| Clustering model | $k$-means | Categorize the raw dataset |

**Regression Models.** The first class of algorithms are the first three CNNs for regression. These are nonlinear regression algorithms. Since we are interested in identifying the two order parameters and the permeabilities, we use CNNs-I, CNNs-II, and CNNs-III with the same structure in Fig. 2. To get a faster convergence, we use Adam algorithm [1] as an optimizer to update parameters and a rectified linear unit (ReLU) $\boldsymbol{a} = \max(0, \boldsymbol{x})$ [2] as an activation function due to nonlinear regression analyses.

**Binary Classification Models.** The next set of machine learning models we consider are the last CNNs for regression. These are nonlinear classification algorithms for identifying a new order parameter and the critical transition point by CNNs-IV with the same structure in Fig. 2. Unlike CNNs-I, CNNs-II, and CNNs-III, we use a sigmoid activation function, $\boldsymbol{a} = 1/(1+e^{-\boldsymbol{x}})$, as an activation function to make sure the outputs are between 0 and 1.

**Generation Models.** Generative models contain a series of models used to randomly generate observable data. These models include Autoencoder (AE), Boltzmann Machines, Restricted Boltzmann Machines, Deep Belief Networks, Deep Boltzmann Machines, Sigmoid Belief Networks, Differentiable Generator Networks, Generative Adversarial Networks, Generative Moment Matching Networks, Convolutional Generative Networks, Auto-Regressive Networks, neural auto-regressive density estimator, Generative stochastic networks, and so on.

In our work, we consider two generation models, i.e., the VAE (Autoencoder, see Fig. 3) and the cVAE (see Fig. 4). Autoencoder (AE, see Fig. S. 1) is the cornerstone of the VAE and the cVAE. The AE is composed with an encoder and a decoder. The encoder and the decoder can be two different CNNs. The connection between the encoder and the decoder is the layer of "Latent", which is the output of the encoder and the input of the decoder. The inputs of the encoder is the each row in $\boldsymbol{X}$ with one dimension. Usually, the output size of the encoder is smaller than the input size. Consequently, the encoder, represented by the encoding function $\boldsymbol{Z} = f(\boldsymbol{X})$, compresses the raw configuration $\boldsymbol{X}$ into latent variable $\boldsymbol{Z}$ that are valid representation for the raw configuration $\boldsymbol{X}$. The output $\hat{\boldsymbol{X}}$ approaches the raw configuration $\boldsymbol{X}$. On the contrary, the decoder, represented by the decoding function $\hat{\boldsymbol{X}} = g(\boldsymbol{Z})$, reconstructs the raw configuration $\boldsymbol{X}$ from the latent variable $\boldsymbol{Z}$. Contrast with the encoder, the decoder is used to transform latent variable $\boldsymbol{Z}$ into higher-dimensional feature $\hat{\boldsymbol{X}}$. Hence, the AE can be formulated by the function $\hat{\boldsymbol{X}} = g(f(\boldsymbol{X}))$. By training the AE, the latent variable $\boldsymbol{Z}$ will possess key information for data reconstruction.

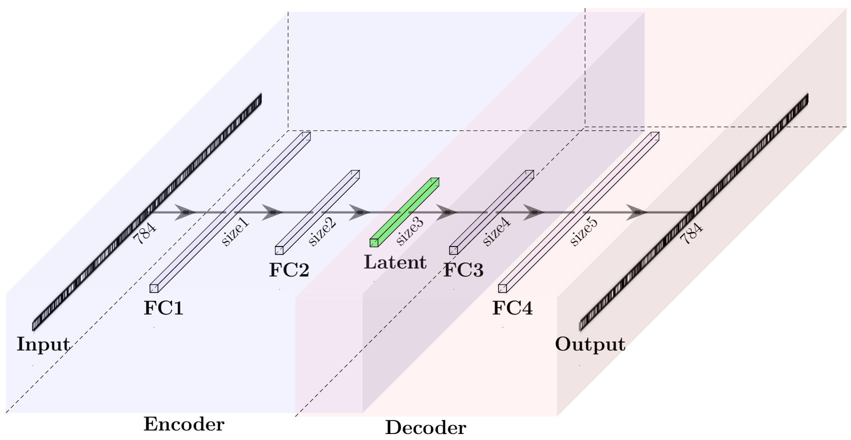


FIG. S. 1: An example of the AE with an encoder and a decoder. The left large light purple cuboid is the encoder with three layers, including "FC1", "FC2", and "Latent". And the right large light red cuboid is the decoder with three layers, including "FC2", "FC4", and "Output". The overlapping green cuboid "Latent" is a fully connected layer with "size3" latent variables. The rectangles with 784 black and white lattice sites represent percolating configuration $\boldsymbol{X}$ on the left and its reconstruction $\hat{\boldsymbol{X}}$ on the right, respectively. The light purple cuboids ("FC1" and "FC2") stand for four fully connected layers with size of "size1", "size2", "size4", and "size5", respectively.

**Dimensional Reduction Model.** In the field of machine learning, dimensional reduction refers to map the configuration $\boldsymbol{X}$ in the high-dimensional space to the low-dimensional space. The essence of dimensional reduction is to learn a mapping function $\boldsymbol{Z} = f(\boldsymbol{X})$. $\boldsymbol{Z}$ refers to the representation of a low-dimensional vector after dimensional reduction. Usually, the dimension of $\boldsymbol{Z}$ is smaller than the dimension of $\boldsymbol{X}$. $f(\cdot)$ may be linear or nonlinear.

The reasons why using the data representation obtained by dimensional reduction are as follows: (1) $\boldsymbol{X}$ with high-dimensional contains redundant information, which causes larger errors in practical applications, such as image recognition; thus, it is possible to reduce the error caused by redundant information; (2) and it is possible to find the intrinsic features of $\boldsymbol{X}$ through the dimensional reduction models. In many cases, the dimensional reduction models become a part of data preprocessing, such as PCA. More information about PCA can be seen in Sec. IIIC.

**Clustering Model.** $k$-means, one of unsupervised learning, is a non-parametric clustering algorithm. $k$-means often exhibit strong performance in problems where a proper category is unknown, and can be relatively implemented by scikit-learn. Here giving the raw configuration $\boldsymbol{X}$, we divide $\boldsymbol{X}$ into $k$ clusters $\boldsymbol{C} = \{\boldsymbol{C}_1, \boldsymbol{C}_2, \ldots, \boldsymbol{C}_k\}$. Let the points within the cluster as close as possible, and the distance between the clusters as far as possible. Our goal is to minimize the squared error $\mathrm{SE}(\boldsymbol{X}_i, \boldsymbol{\mu}_v)$ (see Eq. 1). Where $\boldsymbol{\mu}_v$ $(v = 1, 2, \ldots, k)$ (see Eq. 2) is the mean vector of the cluster $\boldsymbol{C}_v$. There are two caveats. One is that we have to choose a proper value of $k$ by cross validation without prior knowledge. The other is that we have to choose $k$ proper centroids that are not too close. Here we summarize the process of $k$-means algorithm (see Table S. II).

$$\mathrm{SE}(\boldsymbol{X}_i, \boldsymbol{\mu}_v) = \sum_{v=1}^{k} \sum_{\boldsymbol{X}_i \in \boldsymbol{C}_v} ||\boldsymbol{X}_i - \boldsymbol{\mu}_v||_2^2 \tag{1}$$

$$\boldsymbol{\mu}_v = \frac{1}{|\boldsymbol{C}_v|} \sum_{\boldsymbol{X}_i \in \boldsymbol{C}_v} \boldsymbol{X}_i \tag{2}$$

TABLE S. II: The procedure of $k$-means Algorithm

Input: the raw configuration, $\boldsymbol{X}$; the number of the clusters, $k$; the maximum number of iterations, epochs.
Output: the clusters $\boldsymbol{C} = \{\boldsymbol{C}_1, \boldsymbol{C}_2, \ldots, \boldsymbol{C}_k\}$.

1. Randomly select $k$ configurations from $\boldsymbol{X}$ as the initial $k$ centroid vectors $\{\boldsymbol{\mu}_1, \boldsymbol{\mu}_2, \ldots, \boldsymbol{\mu}_k\}$;
2. For epoch $= 1, 2, \ldots,$ epochs;
(a) Initialize the cluster partition $\boldsymbol{C}$, $\boldsymbol{C}_t = \emptyset (t = 1, 2, \ldots, k)$;
(b) For $i = 1, 2, \ldots, M$, calculate the distance $d_{iv} = ||\boldsymbol{X}_i - \boldsymbol{\mu}_v||_2^2$ between $\boldsymbol{X}_i$ and each centroid vector $\boldsymbol{\mu}_v$ $(v = 1, 2, \ldots, k)$, classify $\boldsymbol{X}_i$ corresponding to the minimum value $d_{iv}$ into category $\boldsymbol{\lambda}_i$, and update $\boldsymbol{C}_{\boldsymbol{\lambda}_i} = \boldsymbol{C}_{\boldsymbol{\lambda}_i} \cup \{\boldsymbol{X}_i\}$;
(c) For $v = 1, 2, \ldots, k$, recalculate the new centroid vector $\boldsymbol{\mu}_v$;
(d)If all $k$ centroid vectors have not changed, then go to step 3;
3. Output the clusters $\boldsymbol{C} = \{\boldsymbol{C}_1, \boldsymbol{C}_2, \ldots, \boldsymbol{C}_k\}$.

## II. RESULTS FOR THE CNNS

Here we explore the performance of simulating the two order parametrs by CNNs-I and CNNs-II. The blue lines in Fig. S. 2 refer to the MSE, MAE, and RMSE vary with epochs for training set by CNNs-I and CNNs-II, respectively. And the red lines in Fig. S. 2 refer to the MSE, MAE, and RMSE vary with epochs for testing set by CNNs-I and CNNs-II, respectively. As shown in Table S. III, we get the best CNNs-I and CNNs-II when epoch is 662 and 833, respectively. And the MSE, MAE, and RMSE of the optimal CNNs-I are 0.000818, 0.018294, and 0.028606 for training set, and 0.001806, 0.021274, and 0.042496 for testing set, respectively (see the first row in Table S. III). And the MSE, MAE, and RMSE of the optimal CNNs-II are 0.000315, 0.012202, and 0.017740 for training set, and 0.000772, 0.016134, and 0.027789 for testing set, respectively (see the last row in Table S. III).

In fact, the difference between the blue and red lines represents whether or not the models are overfitting. That is to say, if we create too complex model, the model will be created perfectly, but just for the training data instead of the testing data. In general, the error/accuracy of the training set is slightly smaller/greater than the testing set in Fig. S. 2, 3, 4, 5, 7. Though the differences show that there exist overfitting on our models, it is not enough to affect our conclusions.

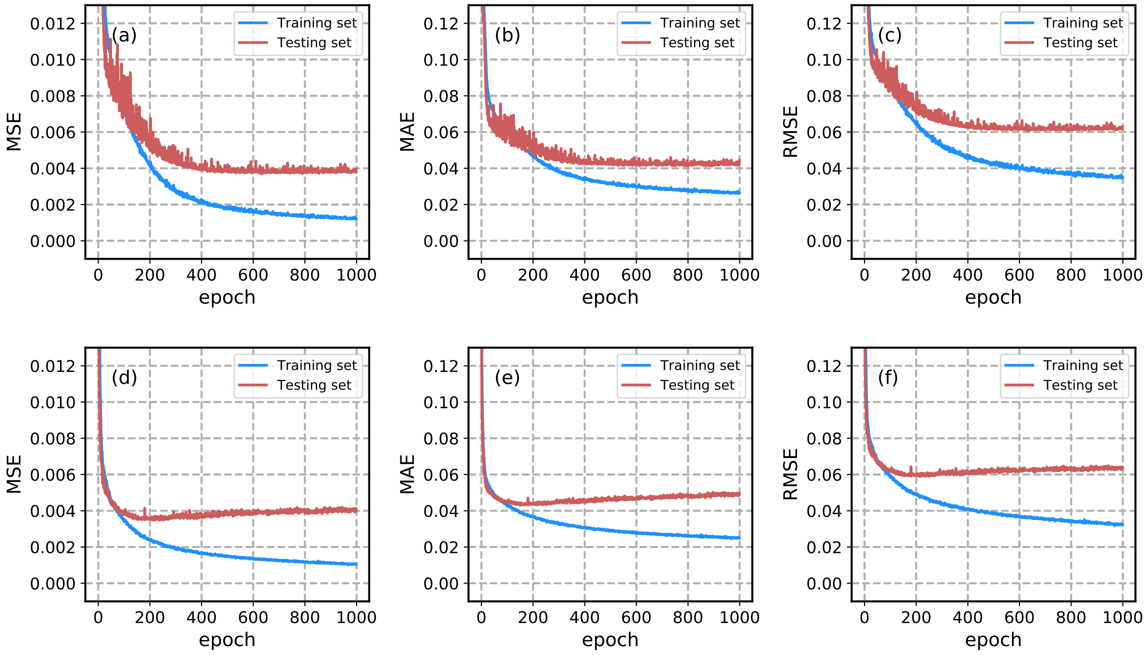


FIG. S. 2: The performance of CNNs-I and CNNs-II. (a-c) The MSE, MAE, and RMSE vary with epochs via CNNs-I, respectively. (e-f) The MSE, MAE, and RMSE vary with epochs via CNNs-II, respectively. The blue and red lines are used for training and testing set, respectively.

TABLE S. III: Results of the optimal CNNs-I and the optimal CNNs-II during the training and testing stages

| Model | epoch | Training | | | Testing | | |
|---|---|---|---|---|---|---|---|
| | | MSE | MAE | RMSE | MSE | MAE | RMSE |
| CNNs-I | 662 | 0.000818 | 0.018294 | 0.028606 | 0.001806 | 0.021274 | 0.042496 |
| CNNs-II | 833 | 0.000315 | 0.012202 | 0.017740 | 0.000772 | 0.016134 | 0.027789 |

Here we explore the extrapolation ability with truncated dataset by CNNs-I. The blue lines in Fig. S. 3 refer to the MSE, MAE, and RMSE vary with epochs for training set by CNNs-I, respectively. And the red lines in Fig. S. 3 refer to the MSE, MAE, and RMSE vary with epochs for testing set by CNNs-I, respectively. As shown Table S. IV, we get the best CNNs-I when epoch is 856. And the MSE, MAE, and RMSE of the optimal CNNs-I are 0.000071, 0.005427, and 0.008450 for training set, and 0.000504, 0.009347, and 0.022452 for testing set, respectively (see Table S. IV).

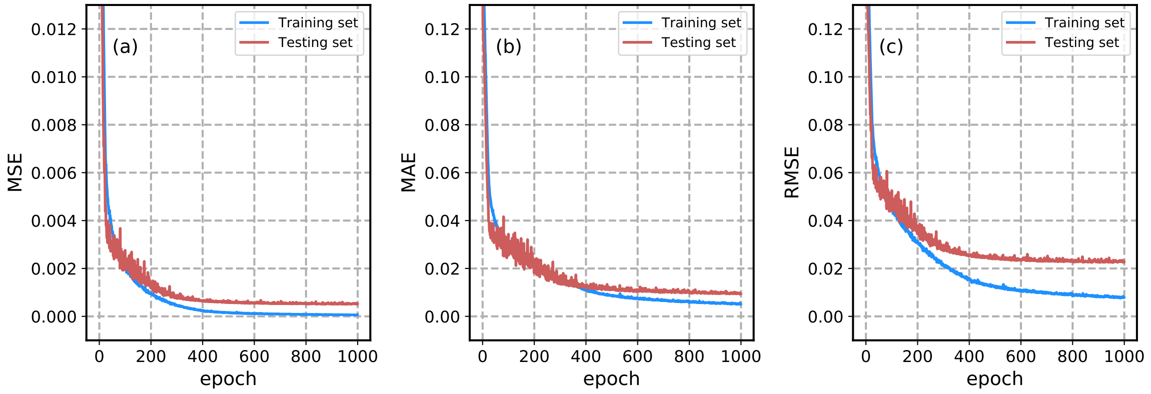


FIG. S. 3: Extrapolation ability with truncated dataset by CNNs-I. (a-c) The MSE, MAE, and RMSE vary with epochs by CNNs-I. The blue and red lines are used for training and testing set, respectively.

TABLE S. IV: Results of the optimal CNNs-I with truncated dataset during the training and testing stages

| Model | epoch | Training | | | Testing | | |
|---|---|---|---|---|---|---|---|
| | | MSE | MAE | RMSE | MSE | MAE | RMSE |
| CNNs-I | 956 | 0.000071 | 0.005427 | 0.008450 | 0.000504 | 0.009347 | 0.022452 |

Here we explore the robustness of CNNs-I and CNNs-II when adding noises (5%, 10%, and 20%) into the two order parameters. The first panel in Fig. S. 4 refers to the MSE, MAE, and RMSE vary with epochs for different noises by CNNs-I, respectively. And the bottom panel in Fig. S. 4 refers to the MSE, MAE, and RMSE vary with epochs for different noises by CNNs-II, respectively. As shown Table S. V, we get the best CNNs-I with different noises when epoch is 634, 370, and 121. The MSE, MAE, and RMSE of the optimal CNNs-I with 5% noise are 0.001531, 0.029299, and 0.039130 for training set, and 0.003730, 0.042500, and 0.061076 for testing set, respectively. The MSE, MAE, and RMSE of the optimal CNNs-I with 10% noise are 0.004754, 0.052782, and 0.068948 for training set, and 0.008440, 0.069633, and 0.091871 for testing set, respectively. The MSE, MAE, and RMSE of the optimal CNNs-I with 20% noise are 0.019483, 0.107892, and 0.139580 for training set, and 0.025276, 0.121460, and 0.158985 for testing set, respectively. The MSE, MAE, and RMSE of the optimal CNNs-II with 5% noise are 0.002538, 0.037629, and 0.050374 for training set, and 0.003461, 0.043311, and 0.058831 for testing set, respectively. The MSE, MAE, and RMSE of the optimal CNNs-II with 10% noise are 0.007155, 0.064488, and 0.084585 for training set, and 0.009680, 0.074368, and 0.098387 for testing set, respectively. The MSE, MAE, and RMSE of the optimal CNNs-II with 20% noise are 0.025883, 0.124777, and 0.160881 for training set, and 0.030106 and 0.134895, and 0.173512 for testing set, respectively.

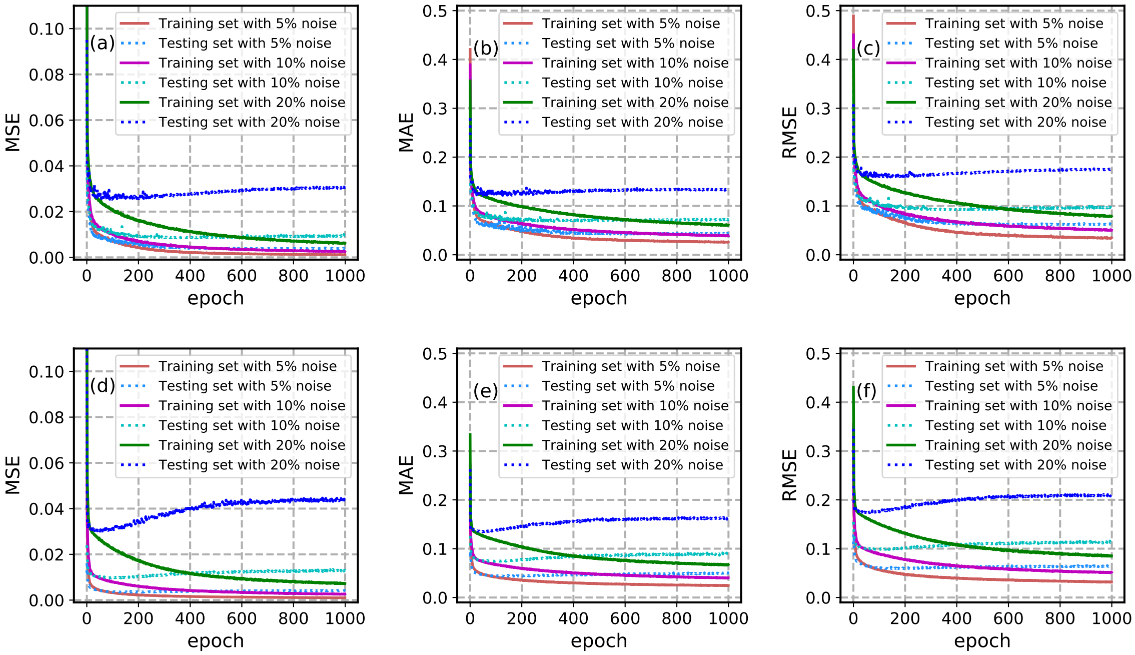


FIG. S. 4: Robustness of CNNs-I and CNNs-II when adding noises into the two order parameters. (a-c) The MSE, MAE, and RMSE vary with epochs by CNNs-I. (e-f) The MSE, MAE, and RMSE vary with epochs by CNNs-II. The blue and red lines are used for training and testing set, respectively.

TABLE S. V: Results of the optimal CNNs-I and CNNs-II with noises (5%, 10%, and 20%) during the training and testing stages

| Model | epoch | Training | | | Testing | | |
|---|---|---|---|---|---|---|---|
| | | MSE | MAE | RMSE | MSE | MAE | RMSE |
| CNNs-I with 5% noise | 634 | 0.001531 | 0.029299 | 0.039130 | 0.003730 | 0.042500 | 0.061076 |
| CNNs-I with 10% noise | 370 | 0.004754 | 0.052782 | 0.068948 | 0.008440 | 0.069633 | 0.091871 |
| CNNs-I with 20% noise | 121 | 0.019483 | 0.107892 | 0.139580 | 0.025276 | 0.121460 | 0.158985 |
| CNNs-II with 5% noise | 160 | 0.002538 | 0.037629 | 0.050374 | 0.003461 | 0.043311 | 0.058831 |
| CNNs-II with 10% noise | 137 | 0.007155 | 0.064488 | 0.084585 | 0.009680 | 0.074368 | 0.098387 |
| CNNs-II with 20% noise | 61 | 0.025883 | 0.124777 | 0.160881 | 0.030106 | 0.134895 | 0.173512 |

Here we explore the performance of simulating the permeabilities by CNNs-III. The blue lines in Fig. S. 5 refer to the MSE, MAE, and RMSE vary with epochs for training set by CNNs-III, respectively. And the red lines in Fig. S. 5 refer to the MSE, MAE, and RMSE vary with epochs for testing set by CNNs-III, respectively. As shown in Table S. VI, we get the best CNNs-III when epoch is 968. And the MSE, MAE, and RMSE of the optimal CNNs-III are 0.000001, 0.000725, and 0.000958 for training set, and 0.000189, 0.010358, and 0.013753 for testing set, respectively (see Table S. VI).

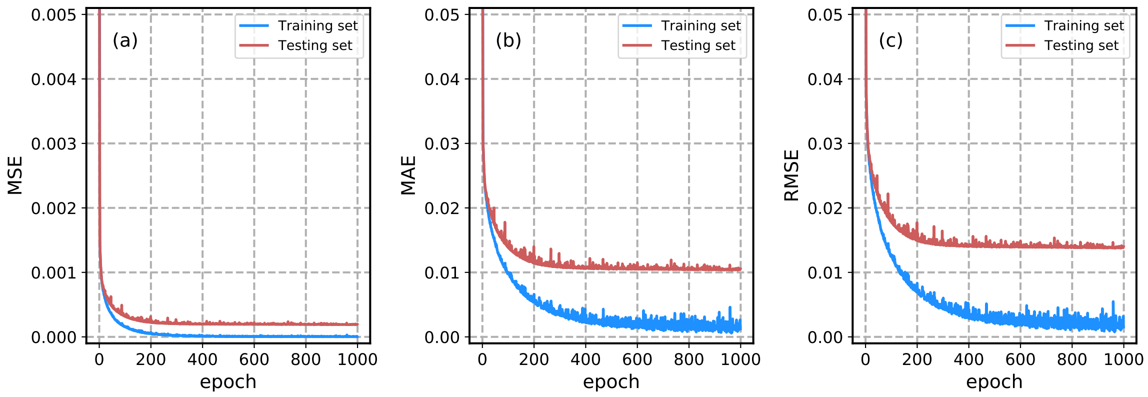


FIG. S. 5: The performance of CNNs-III. (a-c) The MSE, MAE, and RMSE vary with epochs by CNNs-III. The blue and red lines are used for training and testing set, respectively.

TABLE S. VI: Results of the optimal CNNs-III during the training and testing stages

| Model | epoch | Training | | | Testing | | |
|---|---|---|---|---|---|---|---|
| | | MSE | MAE | RMSE | MSE | MAE | RMSE |
| CNNs-III | 968 | 0.000001 | 0.000725 | 0.000958 | 0.000189 | 0.010358 | 0.013753 |

In Fig. S. 6, we explore the robustness of simulating the two order parameters and the permeabilities by the VAE and the cVAE. The blue lines in Fig. S. 6 refer to the loss function, the binary cross-entropy, and the KL divergence vary with epochs for training set by the VAE and the cVAE, respectively. And the red lines in Fig. S. 6 refer to the loss function, the binary cross-entropy, and the KL divergence vary with epochs for testing set by the VAE and the cVAE, respectively. As shown in Table S. VII, we get the best the VAE and the cVAE when epoch is 981 and 954, respectively. And the loss function, the binary cross-entropy, and the KL divergence of the optimal the cVAE are 24.414131, 19.164835, and 5.249296 for the VAE, and 4.130027, 0.838941, and 3.291087 for the cVAE, respectively (see the first row in Table S. VII).

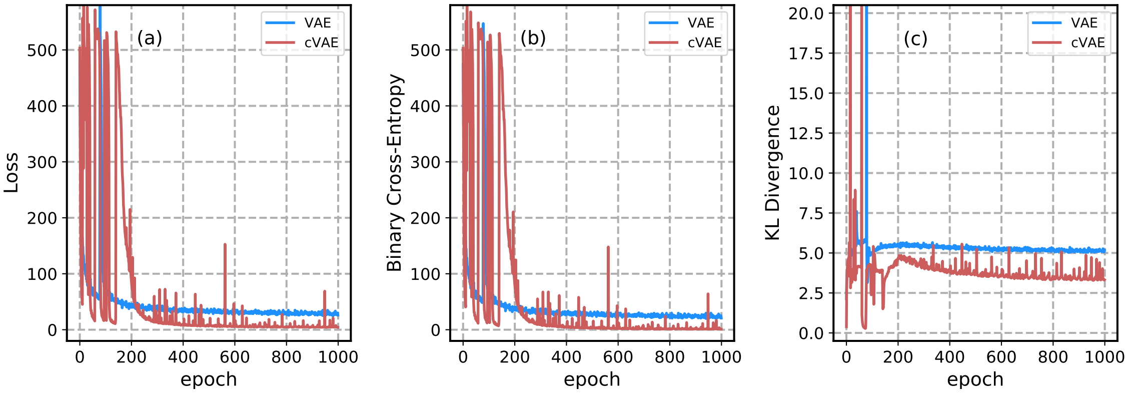


FIG. S. 6: The performance of the VAE and the cVAE. (a-c) The loss function, the binary cross-entropy, and the KL divergence vary with epochs by the VAE and cVAE. The blue and red lines represent the performance for the VAE and the cVAE, respectively.

TABLE S. VII: Results of the optimal VAE and cVAE during the training and testing stages

| Model | epoch | Training | | |
|---|---|---|---|---|
| | | Loss | Binary Cross-Entropy | KL Divergence |
| VAE | 981 | 24.414131 | 19.164835 | 5.249296 |
| cVAE | 954 | 4.130027 | 0.838941 | 3.291087 |

In Fig. S. 7, we explore the performance of deducing the new order parameter and the critical transition point by CNNs-IV. The solid lines in Fig. S. 7 refer to the binary cross-entropy and binary accuracy vary with epochs for training set by CNNs-IV, respectively. And the dashed lines in Fig. S. 5 refer to the binary cross-entropy and binary accuracy vary with epochs for testing set by CNNs-IV, respectively. As shown in Table S. VIII, we get the best CNNs-IV when epoch is 106, 137, 125, 146, 167, 147, 99, 124, 100, 95, and 121, respectively. The binary cross-entropy and binary accuracy of the optimal CNNs-IV with preset value of 0.55 are 0.052304 and 0.979250 for training set, and 0.086404 and 0.962844 for testing set, respectively. The binary cross-entropy and binary accuracy of the optimal CNNs-IV with preset value of 0.56 are 0.056195 and 0.975750 for training set, and 0.088272 and 0.962531 for testing set, respectively. The binary cross-entropy and binary accuracy of the optimal CNNs-IV with preset value of 0.57 are 0.049904 and 0.981500 for training set, and 0.086581 and 0.963188 for testing set, respectively. The binary cross-entropy and binary accuracy of the optimal CNNs-IV with preset value of 0.58 are 0.057224 and 0.978500 for training set, and 0.086191 and 0.962500 for testing set, respectively. The binary cross-entropy and binary accuracy of the optimal CNNs-IV with preset value of 0.59 are 0.055142 and 0.976875 for training set, and 0.086726 and 0.964000 for testing set, respectively. The binary cross-entropy and binary accuracy of the optimal CNNs-IV with preset value of 0.60 are 0.052020 and 0.977250 for training set, and 0.084879 and 0.963687 for testing set, respectively. The binary cross-entropy and binary accuracy of the optimal CNNs-IV with preset value of 0.61 are 0.055771 and 0.976875 for training set, and 0.083742 and 0.964094 for testing set, respectively. The binary cross-entropy and binary accuracy of the optimal CNNs-IV with preset value of 0.62 are 0.052338 and 0.980125 for training set, and 0.084620 and 0.963750 for testing set, respectively. The binary cross-entropy and binary accuracy of the optimal CNNs-IV with preset value of 0.63 are 0.064329 and 0.973375 for training set, and 0.085051 and 0.963094 for testing set, respectively. The binary cross-entropy and binary accuracy of the optimal CNNs-IV with preset value of 0.64 are 0.061360 and 0.974500 for training set, and 0.085749 and 0.963437 for testing set, respectively. The binary cross-entropy and binary accuracy of

the optimal CNNs-IV with preset value of 0.65 are 0.058715 and 0.975375 for training set, and 0.083856 and 0.963375 for testing set, respectively.

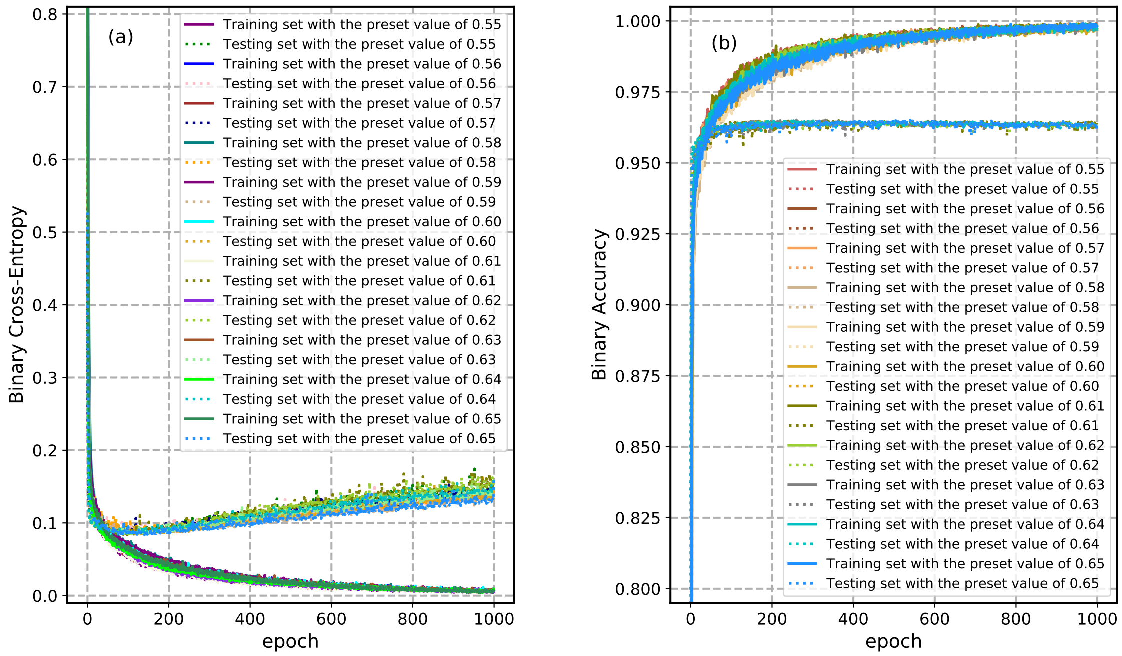


FIG. S. 7: The performance of CNNs-IV. (a-b) The binary cross-entropy and binary accuracy vary with epochs by CNNs-IV. The solid and dashed lines are used for training and testing set, respectively.

TABLE S. VIII: Results of the optimal CNNs-IV during the training and testing stages

| Model | epoch | Training | | Testing | |
|---|---|---|---|---|---|
| | | Binary Cross-Entropy | Binary Accuracy | Binary Cross-Entropy | Binary Accuracy |
| CNNs-IV with preset value of 0.55 | 106 | 0.052304 | 0.979250 | 0.086404 | 0.962844 |
| CNNs-IV with preset value of 0.56 | 137 | 0.056195 | 0.975750 | 0.088272 | 0.962531 |
| CNNs-IV with preset value of 0.57 | 125 | 0.049904 | 0.981500 | 0.086581 | 0.963188 |
| CNNs-IV with preset value of 0.58 | 146 | 0.057224 | 0.978500 | 0.086191 | 0.962500 |
| CNNs-IV with preset value of 0.59 | 167 | 0.055142 | 0.976875 | 0.086726 | 0.964000 |
| CNNs-IV with preset value of 0.60 | 147 | 0.052020 | 0.977250 | 0.084879 | 0.963687 |
| CNNs-IV with preset value of 0.61 | 99 | 0.055771 | 0.976875 | 0.083742 | 0.964094 |
| CNNs-IV with preset value of 0.62 | 124 | 0.052338 | 0.980125 | 0.084620 | 0.963750 |
| CNNs-IV with preset value of 0.63 | 100 | 0.064329 | 0.973375 | 0.085051 | 0.963094 |
| CNNs-IV with preset value of 0.64 | 95 | 0.061360 | 0.974500 | 0.085749 | 0.963437 |
| CNNs-IV with preset value of 0.65 | 121 | 0.058715 | 0.975375 | 0.083856 | 0.963375 |

[1] D. P. Kingma and J. Ba, Adam: A method for stochastic optimization, arXiv preprint arXiv:1412.6980 (2014).
[2] A. F. Agarap, Deep learning using rectified linear units (relu), arXiv preprint arXiv:1803.08375 (2018).
